# Supplementary material for: Synchronization of Multiple Videos
Source: arXiv:2510.14051 source file (2025-10-15)
Supplement: Supplementary file 2 [file fig_joint_alignment.tex]

\begin{figure}[h]

  \centering
  \begin{subfigure}{0.49\textwidth}
  % [left, down, right, up]
    \includegraphics[trim = 5mm 0mm 5mm 12mm, clip, width=\textwidth]{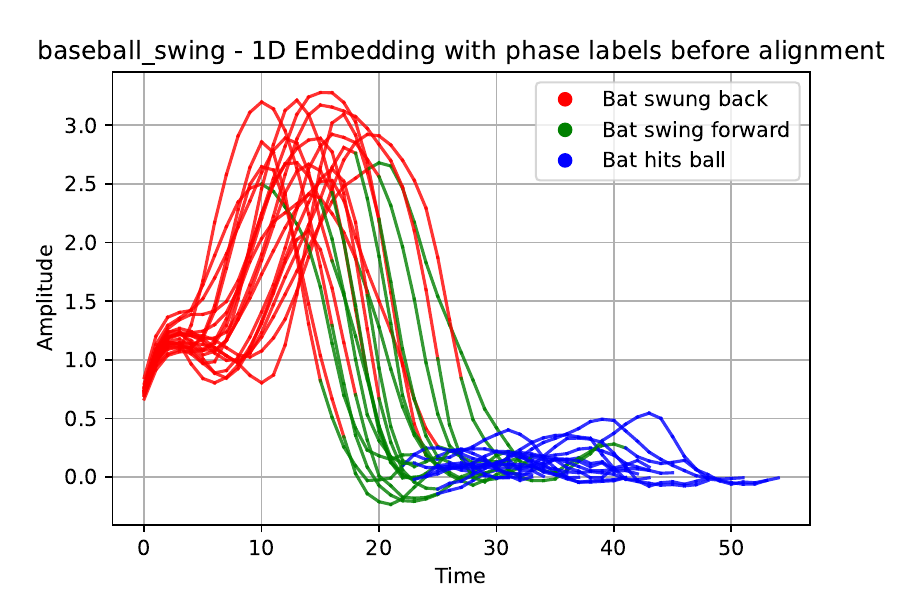}
    \caption{\emph{Baseball swing} 1-D Latent representation}
  \end{subfigure}
  %\hfill
  \begin{subfigure}{0.49\textwidth}
    \includegraphics[trim = 5mm 0mm 5mm 12mm, clip, width=\textwidth]{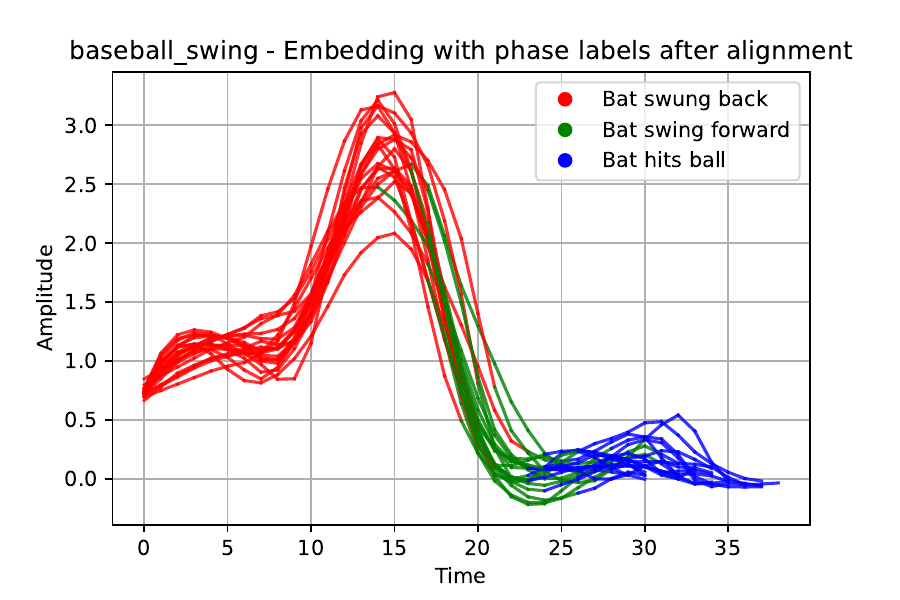}
    \caption{After alignment}
  \end{subfigure}
    \begin{subfigure}{0.49\textwidth}
  % [left, down, right, up]
    \includegraphics[trim = 5mm 0mm 5mm 12mm, clip, width=\textwidth]{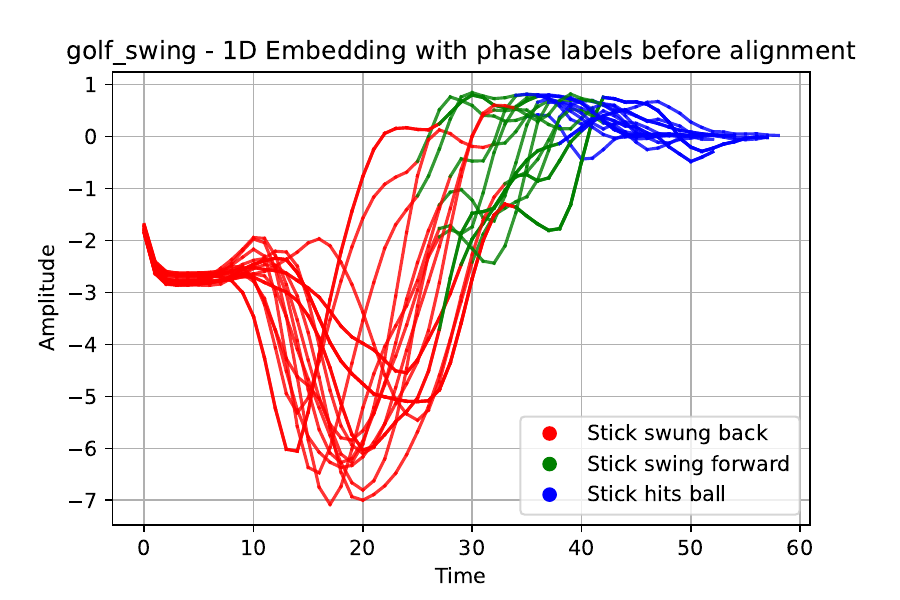}
    \caption{\emph{golf swing} 1-D Latent representation}
  \end{subfigure}
  %\hfill
  \begin{subfigure}{0.49\textwidth}
    \includegraphics[trim = 5mm 0mm 5mm 12mm, clip, width=\textwidth]{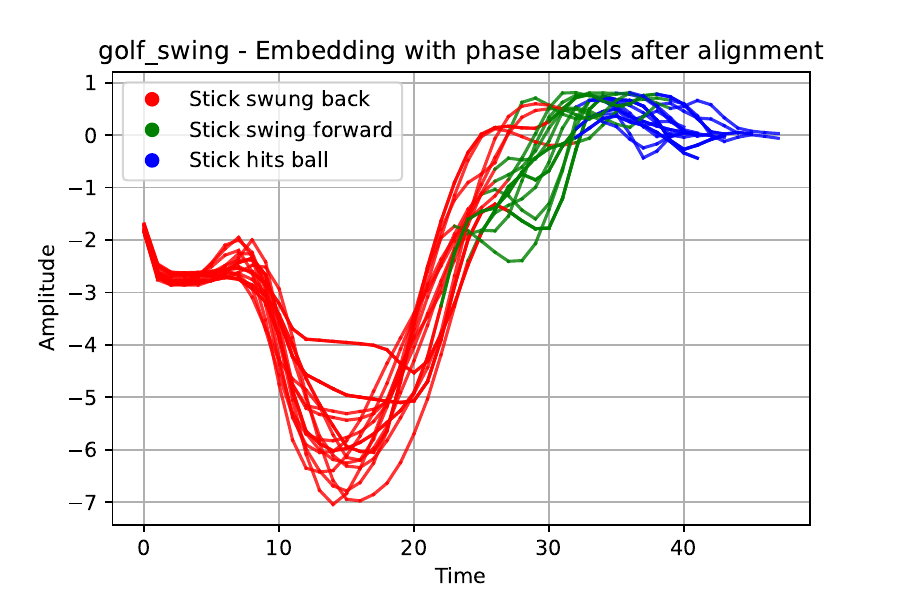}
    \caption{After alignment}
  \end{subfigure}

\caption{Joint alignment of the one-dimensional representation for 20 randomly sampled videos of the \emph{Baseball swing} (top) and \emph{golf swing} (bottom) action colored by the phase labels, before (left) and after alignment (right). }\label{fig:JA:1}

\end{figure}

\newpage
